# Supplementary material for: Correlated Components Analysis - Extracting Reliable Dimensions in Multivariate Data
Source: arXiv:1801.08881 ancillary file (2019-01-20)
Supplement: Supplementary file 1 [file review-and-response.pdf]

December 21, 2018

Dear Reviewers and Editor

First of all, we would like to apologize. This manuscript is much too long. It was intended as a didactic introduction and short collection of new observations on CorrCA. We extended it bit by bit as we received feedback and questions from readers and reviewers, and it has now gotten to be very long. We therefore are deeply grateful for the generous effort of the two present reviewers to have read such a long paper. You have read it with great care and provided insightful comments and questions. Thank you!

To help with the review of this revised manuscript, we have made an effort for this response document to be entirely self contained. The reviewers should know everything that has changed in the manuscript by reading just this document.

Below are reviewer's comments in italic font. Our responses are indented, and text in blue indicates additions to the manuscript. There are additional edits throughout the new manuscript as we have read the entire document one more time for clarity, grammar and spelling.

Best regards,

Lucas, Stefan, Jacek.

Reviewer 1

*I think this is a nice paper, and for the most part very easy to read. There are a few places in particular where I think clarification will be helpful to the reader.*

Thank you for the positive overall evaluation and the thoughtful questions below.

*For the last paragraph on page 8 (begins "The equivalence between CorrCA and LDA..."), would it be possible to describe the intuition by mapping back to the hypothetical data sets (for instance, the dimensions of the tensor for CorrCA)? I think this paper does a really good job of describing the initial hypothetical data setup, and this paragraph in particular could benefit from that clarity.*

We had some text in the manuscript relating LDA that toy example. We reorganized and reworded this text. Hopefully it is more clear now: "The equivalence between CorrCA and LDA is perhaps surprising. **Note that LDA attempts to separate classes so that exemplars of one class do not overlap with the exemplars of other classes. In the illustrative example of Figure 1, time samples  $i$  take on the role of classes. There are 20 classes, each with two exemplars (connected with gray lines). Classes are well**

separated in the direction of component,  $y_1$ , (red arrow), whereas they are overlapping in the original dimensions  $x_1$  and  $x_2$ . Note that the signals are zero-mean across samples but have differing class-means. In this toy example, there is no variance between the two exemplars in each class (vertical lines in panel F indicate that the  $y_1$  values are identical within a class). Thus, CorrCA has found a dimension of the data ( $y_1$ ) in which the classes are perfectly separated. Zero within-class variance leads to infinite separation (Eq. 18) and this in turn to unit correlation (Eq. 22). More generally, what we have demonstrated with Eq. 22 is that increasing separation between samples is equivalent to increasing correlation across samples.”

*This paper shows some examples of CorrCA used in practice, including examples taken from previous literature applying the technique to brain data. A novel aim for the paper is to show that CorrCA can be used with behavioral data for aggregating scores in a way that maximizes inter-rater reliability. While the utility for applying CorrCA to brain data is clear, it is not as obvious to this reader how useful it is to apply CorrCA to the behavioral case. I think this paper could benefit from a discussion of how the results could be used in practice. Specifically, how should a practitioner interpret components that have large weights on multiple variables? One could in some circumstances derive some "story" from the weights (see next paragraph), but it is easy to imagine cases in which a clear story is not easy to derive. What happens in this case? What does it mean for rater-reliability to be high in some linear combination of the variables?*

To provide a motivation we added the following to the section on motor ratings (section 3.2): For many assessment instruments, individual ratings are summed up to obtain a total score. Sometimes one also computes sub-scores by summing over specific ratings that are meaningfully related. In these sums, ratings effectively obtain equal weights, which is a sensible but nonetheless arbitrary choice. CorrCA can suggest weightings that will give the most reliable response across raters, for it should be the goal of any assessment instrument to provide, at a minimum, reproducible results. In this specific example the goal is to find weightings for the 12 motor task that provide reliable aggregate (sub-) scores, and which capture independent aspects of these ratings (independent to second order).

*The "story" version seems to be addressed somewhat in section 3.3, where questions with high weights are examined. The story was one of 'parent involvement' and it was indicated that there was moderate agreement on how independent the children's lives are. Noting that 'parent involvement' is one of the original categories under examination, presumably there are other questions that address in some way 'parent involvement'. CorrCA, like MCCA, looks for greedy directions in the data, and it seems difficult to conclude that, globally, there is moderate agreement on parent involvement, when the conclusion seems to stem from only a small subset of questions that attempt to assess this. Would it be possible to have a table that shows the entire set of questions and the categories that they originally were in?*

The questions are all listed in the a new reference we have added ([Shelton et al. 1996](#)). This is the seminal paper evaluating the Alabama Parenting Questionnaire. The questionnaire can also be found online with a quick google search. [For example here](#). As you can see, there are in fact a few more questions related to this factor.

*Further, in the positive weight direction, only Question 11 is examined. However, looking at Figure 4, it seems Question 41 (if I'm counting correctly) also has a high positive weight, especially compared to the other questions. How did you determine which questions should and should not be made explicit in the manuscript? Especially since there are only 2 questions with a reasonably high positive weight, I don't see why 41 would not be included.*

We had included the strongest 5 questions, regardless of sign. Admittedly 5 is an arbitrary choice. Following your query, we now explicitly list in the paper two more questions that contribute most to this component: “[19. Your child goes out with a set time to be home \(-0.33\)](#); [41. You use time out as punishment \(0.33\)](#) ... The positive correlation of Question 41 with this independence-vs-involvement dimension is interesting as it suggest that this form of punishment is associated with a child's independence.”

*Finally, I don't understand the sentence "Positive weights indicate that the answers should have large scores to increase the value on this aggregate measure (and small scores for negative weights)." I'm assuming by scores you mean the 1 to 5 that is assigned during the test. In the 'standardized' space, low scores (1, 2, etc) will have a negative value, and high scores will have a positive value. This seems to lead to the statement in question.*

There actually is no need to standardize the answers, as this is done already in the definition of ISC. As a result, the output of CorrCA (optimal projection vectors and resulting ISC scores) is invariant w.r.t. changes in the overall mean or scale of the data. The statement cited above is therefore correct. A different question, however, is what kind of statistical relationships between data features (in this case questions) and the aggregate score derived from them can be inferred from non-zero weights; in other words, how model weights need to be interpreted. We already discussed this topic in the section on the forward model. In brief, the backward model provides a recipe on how to linearly combine features in order to optimally extract the correlated component. To achieve this, the backward model needs to amplify the correlated component and at the same time suppress signal contributions that differ between repetitions (here collectively called noise). In practice, it is hard to tell whether a large (positive or negative) weight serves one or the other purpose. An example, in which a large weight is assigned to a pure noise dimension is provided below (gray font). Similarly, cases can be made in which dimensions that are highly correlated with the aggregate score are nevertheless not required to construct that score, and are consequently assigned a (near) zero weight. For these reasons, Haufe et al 2014 argue against interpreting results based on the backward model. It is further argued that, in contrast to the backward model, the forward

model (A matrix) allows one to make valid statements about the statistical relationships between individual features and the compound score. We therefore now report the forward model in this figure and changed this sentence to the following, which is hopefully also easier to understand: “The sign of the forward weights indicate here whether the answer to that question correlate positively or negatively with the aggregate measure (Haufe 2014).”

Note that in other cases the exact relationships between data features and composite scores may be of less interest but it may be desired that correlated components can be constructed from a small set of features/questions. In these cases, an analysis of backward model weights may provide valuable insight on what data features are most important to construct a reliable aggregate measure regardless of whether these individual features are dominated by signal or noise sources. An example of such an analysis is provided in Section 3.2.

We have expanded the section on the forward model to briefly touch on some these issues: “The utility of the forward model will be demonstrated for the case of brain activity, where we are interested in how the activity of a recovered neural source manifests at the sensor level (Figure 2 and Figure 5). These forward models can be used directly to perform source localization to identify the spatial origin of the corresponding current sources (Haufe 2014). In the case of questionnaire ratings (section 3.3) we will interpret the meaning of a component by inspecting the forward model, as it measures the correlation of a component with answers of raters on different topics. For the case of ratings, we may also be interested in which items lead to a reliable aggregate score (sections 3.2). In these cases, an analysis of backward model weights may provide valuable insight on what data features are most important to construct a reliable aggregate measure. Note that if the original data is uncorrelated, then  $R_W$  is diagonal and the projections  $V$  are orthogonal. In that case the forward and backward models are identical, except of an overall scale for each component. In that case, we can directly inspect the backward model, as is customarily done in PCA, which has orthogonal projections and one inspects the component “loadings”. In the example of Figure 3.3 D the covariance  $R_W$  is approximately diagonal and one can inspect the results with either the forward or backward model.”

This is an adaptation of example 1 from Haufe 2014: Imagine the case were there are two psychological constructs, C1 and C2. C1 could be interest in the topic of a lecture and C2 could be motivation to pass the exam. Now imagine question Q1 touches both of these concepts: “How likely is it that you will attend tomorrow’s lecture?” This could be modeled as  $Q1 = C1 + C2$ . Q2 may simply ask “How motivated are you to pass the exam on the topic?”, which could be modeled as  $Q2 = C2$ . Assume that C1 and C2 are uncorrelated (i.e. interest is independent of whether a lecture is mandatory or optional), but C1 is more reliably expressed across raters than C2. Then the first CorrCA component will need to approximate C1, which is relatively easily achieved as  $C1 = w1 * Q1 + w2 * Q2$  with  $w1 = 1$  and  $w2 = -1$ . However, despite the significant negative weight, Q2 is not negatively correlated or in any other way statistically related to the aggregate measure that

is C1. There is only a conditional dependence between Q2 and C1 through Q1, which is however not of interest or at least does not afford the interpretation that Q2 measures interest (C1), because it is in fact measuring motivation (C2), which is an orthogonal construct. The conditional dependence between Q2 and C1 given Q1 is however exploited by CorrCA to remove the influence of C2 on Q1.

*However, this goes against my intuition of how this algorithm works. Consider the following example. Consider two questions in the survey. Generate two sets of scores in the standardized space that are uncorrelated with each other, call them set 1 and set 2. For question 1, assign parents the standardized scores of set 1, and the children the standardized scores of set 2. For question 2, assign the parents the the standardized scores of set 2 times -1, and the children the standardized scores of set 1 times -1. For each question, these scores are uncorrelated. However, when you add the scores for question 1 to the negative of the scores of question 2, this linear combination has correlation 1. First, this example seems to (without further exploration of the data) contradict the statement about positive scores corresponding to high values etc. Could you please clarify what you mean by the statement in question?*

In this example, positive scores in question 1 do in fact lead to larger values in the sum aggregate score. And negative scores in question 2 (small values prior to standardization) will also increase the sum. So we are not sure we see the conflict. At any rate, we reworded it above, which hopefully is more clear.

*Second, this example possibly illustrates that (again without further exploration of the data) it need not be the case that (in the previous paragraph of this review) parents and children necessarily need to agree in the dimension of 'parent involvement', but rather that there is some linear combination in which their aggregated responses are highly correlated. Am I interpreting this incorrectly?*

Correct, it is possible that the questions are formulated such that parents and children do not agree in each individual question, yet, once combined the two agree exactly. The hypothetical example constructed by the reviewer would suggest that the difference between the two questions is the relevant dimension. We simulated this example and display it below analogously to Figure 1 of the paper.

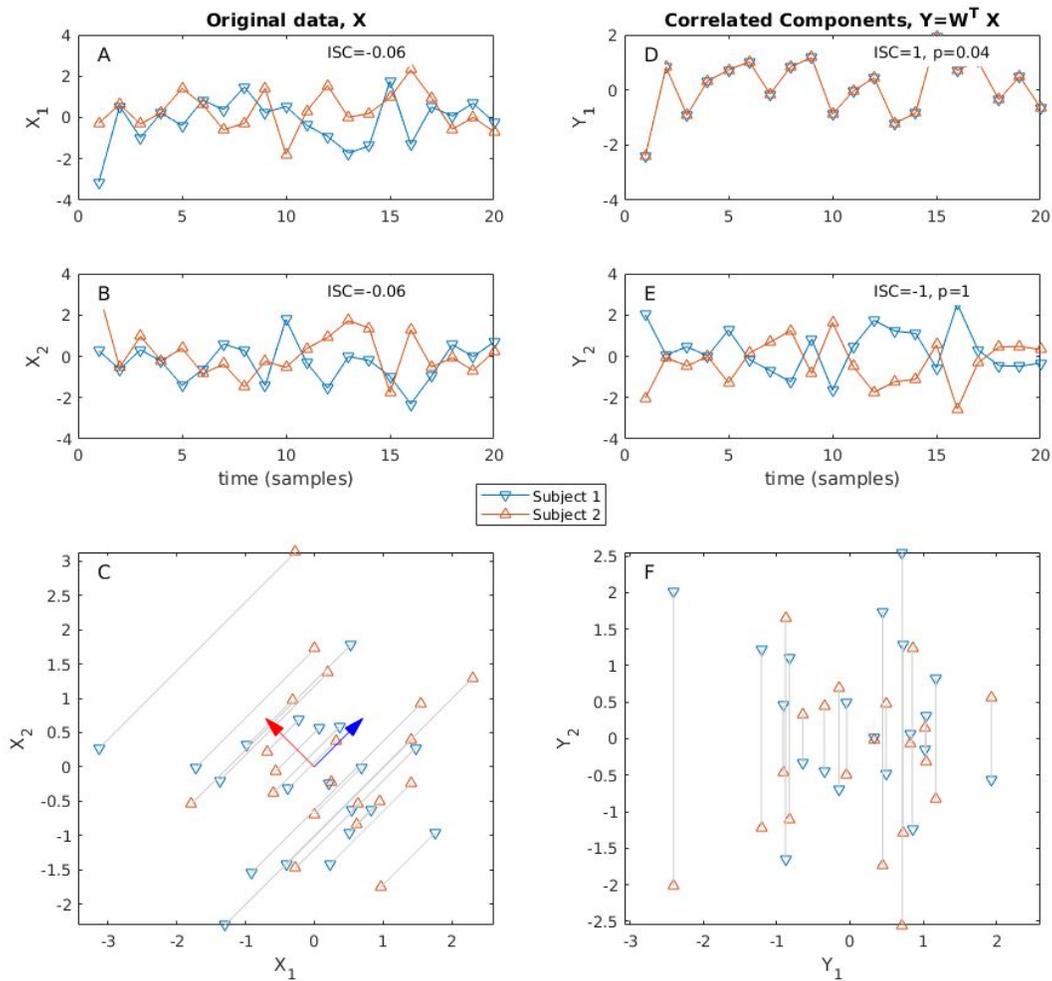

In the example provided above the difference of two answers could provide a good estimate for the construct “interest in the lecture”. In the Alabama Parenting Questionnaire the correlation with some questions and anti-correlation with other is a fairly good indication that the dimension refers to the level of child independence vs parent involvement.

*Minor point: there seems to be a word missing in the second sentence of the paragraph on page 2 that starts with "More generally".*

Thanks for catching that. The missing word was “data”.

Reviewer 2

*The authors describe a reasonable and interesting extensions to canonical correlations analysis (CCA) for handling data across multiple subjects. They have published the basic idea in prior work but this paper aims to provide a comprehensive and didactic introduction to the method. I think this makes a useful contribution to the field.*

Thank you for the positive evaluation, and the detailed comments below.

*Their method CorrCA can be thought of as similar to CCA except the weights producing the low-dimensional representation of the data are constrained to be the exact same for each subject. This is a stronger constraint than CCA or multi-way CCA in which each subject gets its own set of weights. Thus, CorrCA will be most useful in cases where the measurements made on each subject are congruent — CorrCA may work on EEG electrodes which have a standardized location on each subject, but it won't work on direct neural recordings across subjects (neuron  $i$  in subject 1 typically has no special relation to neuron  $i$  in subject 2). Nonetheless, by including this stronger assumption the model can be more informative in these specialized circumstances.*

*I really like this paper. However, the presentation of the model and its application to data are rather dense and difficult to read in spots. Since the contribution of this paper seems to be mostly pedagogical (with some new observations about the model) I've made detailed comments about the conceptual clarity of the paper with the hope that the authors will revise and resubmit.*

*Conceptual comments:*

*(1) Equivalence of Linear Discriminant Analysis (LDA) and CorrCA. One of the novel contributions of the paper is the observation that corrCA is equivalent to LDA when comparing groups that have equal means. While this is interesting, the practical significance of this is not clear to me. I did not much conceptual insight from this section.*

The benefits are mostly mathematical. For instance, by linking to the established F-statistic one obtains a strict parametric test of significance. We say this now right after establishing the link between ISC,  $\rho$ , and separation  $S$ : [“This relationship will be useful in Section 2.4 where we establish a link between ISC and the classic F-statistic \(Eq. 26\), which yields a parametric test for statistical significance of ISC.”](#)

We also tried to improve the section that explains the conceptual relationship for CorrCA and LDA (see new text in response to your first question above).

*(a) The author's mention that CorrCA can be extended to non-linear mappings using standard kernel methods -- but to me this is clear without needing to draw the connection to LDA (equation 8 is already very close to a compatible formulation!). Also kernel-CCA has been described before.*

We should have cited kernel-CCA, which was an oversight that we have now corrected by adding: “Note that a similar result is obtained for the kernel version of CCA, namely, the conventional CCA algorithm is applied to kernel matrices instead of the original data (Lai et al. 2000).” Maybe one could have derived kernel-CorrCA without alluding to LDA first. But as a matter of fact, the analogy inspired and helped us to derive the kernel version. To us it is less clear how to directly derive kernel-CorrCA from kernel-CCA.

*(b) It is unclear to me that LDA works very well if all the groups have equal means. Especially in the case of having two classes -- the normal vector to the decision boundary is  $\text{inverse}(\Sigma) * (\mu_1 - \mu_2)$  which is uninformative when  $\mu_1 = \mu_2$ . If LDA is only equivalent to corrCA in this degenerate case, does it really matter?*

Sorry, this is a misunderstanding. We have added the following clarifications: “Note that equal sample-means,  $\bar{x}_*^l = \bar{x}_*^k$ , does not imply equal class-means,  $\bar{x}_i^* = \bar{x}_j^*$ . Zero-mean signals will naturally satisfy this condition and will typically still have different class means.” and later where we explain Figure 1: “Note that the signals are zero-mean across samples but have differing class-means.” To avoid this confusion we now talk in the paper mostly about “zero-mean signals” instead of “equal mean”.

*(c) It should be mentioned that LDA doesn't require equal number of samples in the various classes, whereas corrCA does have this requirement (if I understand the model correctly).*

That is correct, we added: “Notice that the equivalence between CorrCA and LDA requires the same number of exemplars in each class -- something that is not usually the case in conventional LDA. In fact, there is a one-to-one link between exemplars across classes (gray lines in panels C and F of Figure 1).”

*(2) Comparison to CCA. The authors compare and explain the differences between corrCA and multi-class CCA (MCCA), but single-class CCA is not mentioned much. Not all readers may be familiar with CCA, so I wonder if it would be worth adding a section that explains when to use CCA vs. MCCA vs. corrCA. If one has N subjects, one can still compute CCA between all pairs of subjects and this would give you a different view on your data than fitting a single MCCA class. Performing classic CCA on individual pairs might be useful in experiments involving paired observations (e.g. age-matched subjects in control group vs experimental group). Do the authors agree that this is another interesting baseline model to discuss?*

Matched controls seems like a good application of CCA. We are not familiar with applications of pairwise CCA in the case that there are more than  $M=2$  datasets. All publications we have seen with  $M>2$  use MCCA, which is understandable as it would be difficult to interpret  $M*(M-1)/2$  model pairs that such pairwise CCA would yield. MCCA yields instead  $M$  models and is thus easier to interpret. We hesitate expanding on these topics as we want to keep the paper focused on CorrCA. We have already added more

material on MCCA than we had ever envisioned.

(a) If I understand correctly, CCA would find the same result that is shown in figure 1. However, maybe in the presence of noise corrCA would do better? Would it be possible/useful to explain the differences between CCA, MCCA, and corrCA in this simple example?

Actually, when we run CCA on this data we get identical result for component 2, but not for component 1. The corresponding forward models are shown here for one example (the exact result depend on the specific (random) data).

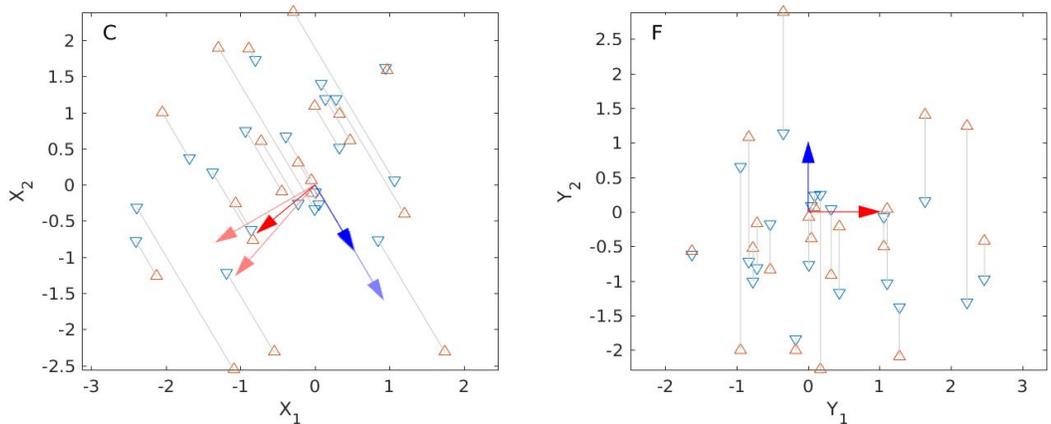

The dark shaded arrows are the two components for CorrCA. The light shaded arrows are the results for CCA (MCCA with  $M=2$ ). There are two light-red, one for each subject (the two light-blue overlap exactly). We considered including this in Figure 1 of the paper, but decided against it, as some sample readers of this figure got confused at that point of the presentation with all these arrows. Instead we write at the end of section 2.6: “In the illustrative example of Figure 1, CorrCA by definition gives the same result for both subjects (red and blue arrows), but we find that the directions derived with CCA differ between subjects (not shown).”

(b) I believe MCCA and CCA are equivalent in the  $N=2$  case (e.g. Zurich Neuromotor Assessment example) and it would be worth noting this throughout the manuscript.

We added the following: “When there are only two data sets ( $M=2$ ) then the present MCCA algorithm reduces to conventional CCA (Borga 1998, see Table 4.1) .... In section 3.3 we will apply CCA to ratings data from two distinct raters (pairs of parent and child), in which case distinct projections may be warranted.” We also clarify earlier “However, in the case of diverse subjects or raters it may make sense to assume that each should receive their own projection vectors. For instance, brain activity recorded at a specific location may differ between subjects because of anatomical or functional differences.

This brings us to the case treated by Canonical Correlation Analysis (CCA) for  $M=2$ , or more generally, multi-set CCA (MCCA) for  $M>2$ ."

*(3) Assumptions of corrCA. One of the most insightful comments in the paper comes on page 24, right before the conclusion "Identical covariance structures of signal and noise components across subjects are a fundamental assumption of corrCA..." Since this is buried deep in the paper, I would suggest including a similar sentence in early sections of the paper (ideally with less jargon, or with an example that less technical readers could relate to).*

In an effort to use less jargon we now specify this assumption in terms of shared directions  $A$ . We added also some language to clarify how these simulations presented here are to be interpreted. "Significant drops in the number of estimated correlated components as well as the average ISC are observed if the signal directions, the noise directions, or both, differ across subjects. Note that varying directions of the non-reproducible component  $A_n^1$  across subjects is equivalent to adding noise, so that the dependence on the noise directions shown in Figure~10 (panel C & D) is a restatement of the dependence on SNR of Figure 7. This result illustrates that identical directions for the signal components across subjects is a fundamental assumption of CorrCA." And in the text related to Figure 1 we have added: "It is important to note that while both directions are shared by the two subjects, only one of these dimensions expresses a common waveform.... The fundamental assumption of CorrCA is that there is a reproducible signal and a non-reproducible noise, and that the directions of the reproducible signal are shared between subjects."

*Technical comments:*

*(1) Comparison to multi-class CCA (MCCA). The authors show a couple examples where corrCA outperforms MCCA. MCCA performs badly in these cases because it has more parameters and overfits the data. However, my understanding is that it is relatively easy to regularize MCCA using the same methods that the authors use to regularize corrCA. While MCCA may need stronger regularization than corrCA in many cases, that doesn't mean MCCA doesn't perform just as well if this regularization is present. It would be a much stronger result if the authors showed that corrCA identified different features of the data than regularized MCCA.*

Correct, one can use the same regularization methods. We now tested this on the first example with EEG from  $N=18$  subjects and replaced the results in Figure 2 with a regularized version of MCCA. In the caption we write now: "Here MCCA was regularized with TSVD ( $K=12$ ; see Appendix C), while CCA was not regularized." In the text we now write: "Indeed, when evaluating ISC on unseen test data the ISC drop substantially for MCCA as compared to the training data, and CorrCA yielded higher ISC values than MCCA for 4 of the first 5 dimensions (Figure 2 B). Both of these findings are indicative of over-fitting in MCCA, despite the use of regularization. We used the Truncated Singular Value Decomposition (TSVD, similar to what is described in Appendix C) and selected a

subspace of  $K=12$  dimensions as this gave the largest cross-validated ISC (summed over the first 3 components). Note that MCCA fits a model for each subject. In this example it uses 216 parameters per component ( $N=18$  subjects,  $K=12$  dimensions), whereas CorrCA uses  $D=64$  parameters per component on these data. While stronger regularization of MCCA is possible, the regularization is ignorant of the shared dimensions, which explains why ISC dropped with stronger regularization on these test data. CorrCA can be seen as a form of regularization that addresses over-fitting, without removing dimensions that significantly correlate between subjects.”

*(2) Cross-validation and statistical significance testing. It seems like there are two reasonable ways to cross-validate corrCA. Either one may leave out time points (along the "T"-dimensional axis) or one may leave out subjects (along the "N" dimensional axis). Can the authors make it clear which was done? It seems like this was usually done across timepoints but in Figure 5 individual trials were left out? What are the practical differences between these two cross-validation strategies?*

Figure 5 does not do any cross-validation, but Figure 4 does, and there we are leaving out parent-child pairs, which in this case takes on the role of samples  $i$ . Therefore cross-validation is done always by leaving out time-points (samples  $i$ ), and in no case by leaving out trials/subjects. We added the following as clarification and motivation for this approach: “Here and in the following examples we computed model parameters  $\mathbf{v}$  by leaving out samples  $i$ , and measured test-set ISC on the left-out samples. The alternative could have been to leave out subjects. However, the number of entries in the between-subject correlation matrix  $\mathbf{R}_B$  defined in Eq. (6) scales quadratically with the number of subjects  $N$ , but linearly with number of samples  $T$ . Thus, we expect the accuracy of  $\mathbf{R}_B$  and the resulting eigenvectors  $\mathbf{v}$  in Eq. (8) to decrease faster when removing subjects instead of samples.”

The issue of statistical significance is described in detail in Appendix D and evaluated with simulations in section 4, i.e. after many of these examples. We do not want to move this somewhat dense technical material forward so as to avoid clutter in the presentation. Instead, we have added a forward reference to alert the readers of this: “We will leverage this observation when we perform tests for statistical significance of  $\rho$  evaluated for independently and identically distributed test data. For non-independent samples, which are more typical of the temporal signals of interest, we will rely instead on shuffle-statistics, which can also be applied directly to training data (see Appendix D). Both method will be evaluated for accuracy in section 4.”

*(3) Time warping limitations. Taking figure 5 (EEG in a single subject) as an example: suppose there were only one dimension that was strongly correlated across trials. If that one feature (time course) was jittered in time on each trial, i.e. occurred with a variable delay, then this would lead to having multiple correlated dimensions. Can this limitation be discussed? I believe a*

*signature of this phenomenon would be that the components extracted by corrCA would be temporal derivatives of each other.*

It is true that, using instantaneous correlation as the optimality criterion, CorrCA does not model time shifts between signals. The presence of time shifts therefore degrades its performance. In the case mentioned by the reviewer, where the correlated signal has a different temporal jitter in each repeat but channels within one repeat are affected by the same jitter, still only one correlated dimension would be found. Only if, in addition, different channels within repeats are also affected by different jitters, the correlated signal would be split into different correlated components, because different linear combinations of the channels would be optimal for different average jitters (i.e. there might be one component being representative for jitters distributed around  $J_1$ , another one for jitter distributed around  $J_2$ , and so on).

In both cases, the ISC/IRC would drop in the presence of jittered signals. The extent of this decrease would strongly depend on the distribution of the jitters in relation to the autocorrelation spectrum of the correlated signal. If most jitters are small enough so that the jittered signals are still significantly positively correlated with each other, then the observed drop will be moderate. If, however, some of the jitters fall into ranges in which the correlation across repeats is near-zero or even significantly negative (which is not unlikely for signals with high frequency content), then this will have more adverse effects, as positive and negative correlations between repeats will cancel each other out in the CorrCA cost function, which in turn will greatly impede the discovery of the correct correlated dimension and reduce the ISC/IRC along that dimension.

In sum, whether CorrCA can be used for jittered signals depends on the properties of the specific data analyzed. For the general case, Fourier-based extensions allowing for random shifts could be considered; such extensions are, however, beyond the scope of this paper.

We have added the following summary on this topic at the end of the section discussing Figure 5 (we have kept it short as the paper is already very long): “[Like most data decomposition algorithms, CorrCA does not require that the underlying data have any time structure. For time series data, this implies that the correlated signal of interest is observed with the same delay in each channel and repetition. If this assumption is violated, drops in performance will occur.](#)”

*(4) Identifiability limitations. I like Appendix A3 and am a bit worried that the small gap between eigenvalues (e.g. Fig 4 B) would lead to identifiability problems. Can this be assessed in the data via cross-validation? For example, are the barely significant components less stable when tested on different subsets of the data? Is this how the error bars are computed in e.g. Fig 4G? I would appreciate a few sentences discussing this point in the main text.*

We agree. This is why we only analyzed the first component in Figure 4. In the discussion of the figure we added: “[We did not analyze subsequent components due to the proximity of residual eigenvalues \(Figure 4, panel C\) and noise may no allow accurate identification \(see section 4.1\).](#)” The error bars are explained in the caption of

figure 5 as follows: “Red error bars indicate the standard deviation across 100 random partitions of the data into training and test sets, and sampling with replacement within that (bootstrap estimates).” As to further discussion, note that section 4 is largely devoted to validation of the method, including identifiability. We direct the reader to this in Section 2: “A thorough evaluation of the conditions under which the algorithm identifies the correct projection vectors  $\mathbf{v}_d$  will be presented in section 4.1 (Fig. 7). The main finding is that the shared waveforms (signal) need to project in the same direction across subjects. Performance degrades if there is additive noise, or equivalently, if the directions of the non-reproducible waveforms (noise) differ between subjects.”

*Minor comments/suggestions on the text:*

*On page 1/2 it would be helpful to define what is meant by "congruent repetitions" and "repeated measurements" more explicitly. For example, you could emphasize that EEG sensors are placed in standard locations across subjects and are thus comparable. When I first read the introduction I did not understand how corrCA was different than vanilla CCA. Again, I think having a couple sentence to contrast your motivations with CCA would be useful.*

We write now: “... where  $N$  are repeated measures with the same sensors ... The methods differs in that CorrCA uses a single set of linear projections for all data sets assuming the repeated measures are all taken in the same space, whereas CCA and MCCA yield a different set of projection vectors for each data-set.”

*Second paragraph page 2. Replace "MCCA" with "unregularized MCCA" to emphasize that your method outperforms in a setting where data is scarce?*

Done.

*Consider replacing " $i = 1 \dots T$ " with " $t = 1 \dots T$ " throughout the notation?*

We thought about this at the outset. The advantage of using  $t$  for time instead of  $i$  is obvious. The issue is that in some applications  $t$  does not index time but individuals (parent/child). Also, in LDA, index  $i$  is used for exemplars, which is what we use it for here. By using  $i$  the notation between CorrCA and LDA is kept consistent. As much as we would like to use  $t$  ourselves, we decided to stick with index  $i$ .

*Equation 9 - I would move  $\rho$  to the front of the right hand side of the equation. Right now it looks a bit like a subscript (" $\mathbf{v}_\rho$ ").*

Done.

*Distinction between IRC and ISC is confusing. Consider just picking one and sticking with it?*

Mathematically they are the same. Prompted by this remark, we considered using just one of the two terms, but decided instead to improve the text in a few relevant places to clarify their use. The problem is that ISC would be a confusing term to use when the repeats are not subjects, but just repeated trials, as in Figure 5 or 3C. On the other hand, using the term IRC throughout would be a problem as ISC is a widely used term in neuroscience applications and we would really like to appeal to it.

On page 5, "Similar to the constraints imposed by Independent Components Analysis (ICA)". I would delete this because statistical independence is not always the same as de-correlation. Also statistical independence typically enters into ICA through the objective function, not a hard constraint.

Most ICA algorithms "sphere" the data as first step, including those that use an objective function. This is done to strictly enforce uncorrelated components. It is a necessary but not sufficient condition of independence, and one that is often implemented directly as a constraint.

Page 7, "see Table 2". Is this meant to say "see Table 1"?

We did mean Table 2. We clarified this by adding that table 2 is in [Appendix G.1](#).

Page 8, "increasing separation between samples is equivalent to increasing correlation across samples." Is there a subtle distinction between "across" and "between" here? If not, I'd just say "increasing separation is equivalent to increasing correlation across samples."

We find that "increasing separation between" is more clear than "increasing separation across". So we would like to keep as is.

Page 10, consider adding a citation to "General Linear Modeling" and noting the difference with generalized linear models (a common confusion).

We added a reference.

Equations 32 and 33 - again, I would move the scalar to the front of the right hand side (similar to equation 9).

Done.

Page 14 - "it is evident that test-retest variability is somewhat higher than the inter-rate variability". Is this meant to be "test-retest variability is somewhat lower than..."? I got confused because the y-axis is correlation, not variability.

Sorry, yes, here we meant to say “[reliability](#)” instead of “variability”. Fixed now.

Figure 5 - Does corrCA provide an easy method for determining which trials were errors vs which were correct?

We added the following for clarification on this point: “[In our earlier work we specifically looked for a projection that distinguishes the EEG evoked response between error and correct responses \(Parra et al. 2000\). Here the goal is to identify reliable error responses.](#)”

I recommend citing the book chapter by De Bie, Cristianini and Rosipal, "Eigenproblems in Pattern Recognition." Which I've found very useful on these topics.

We added reference to this Chapter in the context of kernel methods and in the context of CCA.
